# Supplementary material for: Interpreting a concurrent $\lambda$-calculus in differential proof nets (extended version)
Source: arXiv:2102.05736 source file (2021-02-10)
Supplement: Supplementary file 1 [file appendix.tex]

\newpage
\appendix
\section{Proof nets}
\label{appendix:nets}

We prove in detail various results stated in section~\ref{section:nets}.

\subsection{Swapping (Lemma~\ref{lemma-nets-swapping})}

\begin{proof}\ref{lemma-nets-swapping}
  By induction on both the length of the reduction $\mathcal{S} \leadsto^\ast
  \mathcal{R}$ and $\mathcal{R} \to^\ast \mathcal{R}'$. We consider the
  fundamental case where both reduction are one step : 
  
  \begin{center}
    \begin{tikzpicture}
      \matrix (m) [matrix of math nodes,row sep=3em,column sep=4em,minimum
        width=2em] 
      {
        \mathcal{R} & \mathcal{R}' \\
        \mathcal{S} & \\
      };
      \path[-stealth, auto]
        (m-1-1) edge (m-1-2)
        (m-2-1) edge[equiv1step] (m-1-1);
    \end{tikzpicture} 
  \end{center}

  Consider the following remarks.
  \begin{itemize}
    \item As $\leadsto$ reduction happens inside boxes and $\red{diff}$ outside,
      we can put in a one-to-one correspondence the boxes at depth 0 - and thus
      the $\red{diff}$-redexes - of $\mathcal{R}$ and $\mathcal{S}$ 
    \item If the reduction in $\mathcal{R}$ does not involve a box, it does not interact with
      $\leadsto$, and the diagram can be closed as a square with one step reduction in every
      direction
    \item If it erases a box, we can erase the corresponding one in
      $\mathcal{S}$, which may delete $\leadsto$ redexes or not.  In any case we
      can reduce $\mathcal{S}$ to $\mathcal{S}'$ in one step by erasing the same
      box, where $\mathcal{S}'$ is either $\mathcal{R}'$ or can be reduced to it
      in one $\leadsto$ step if the $\leadsto$ happened in a different box.
    \item If it opens a box, opening the corresponding one in $\net S$ it may turn $\leadsto$-redexes at depth $1$ to
      $\red{diff}$-redexes, as they now appear at the surface. In any case, we
      can close the diagram by peforming either one $\red{diff}$ step followed
      by one $\leadsto$ step, or two $\red{diff}$ steps.

    In the cases listed above, the length of the reduction between
    $\mathcal{R}'$ and $\mathcal{S}'$ never exceeds one, hence we can always
    fill the following diagram :
      
      \begin{center}
        \begin{tikzpicture}
          \matrix (m) [matrix of math nodes,row sep=3em,column sep=4em,minimum
            width=2em] 
          {
            \mathcal{R} & \mathcal{R}' \\
            \mathcal{S} & \mathcal{S'} \\
          };
          \path[-stealth, auto]
            (m-1-1) edge (m-1-2)
            (m-2-1) edge[reduceto] (m-2-2)
            (m-2-1) edge[equiv1step] (m-1-1)
            (m-2-2) edge[equiv01step] (m-1-2);
        \end{tikzpicture} 
      \end{center}
    
    Where the bottom line does not involve duplication.

    .$\mathcal{S}' \underline{\leadsto} \mathcal{R}'$ if $\mathcal{S}' =
    \mathcal{R}'$ or $\mathcal{S'} \leadsto \mathcal{R}'$.

    \item Duplication is the only reduction that can create new
      $\leadsto$-redex. But it requires only one $\to$-step in $\mathcal{S}$.
      This corresponds to the following diagram
      
      \begin{center}
        \begin{tikzpicture}
          \matrix (m) [matrix of math nodes,row sep=3em,column sep=4em,minimum
            width=2em] 
          {
            \mathcal{R} & \mathcal{R}' \\
            \mathcal{S} & \mathcal{S'} \\
          };
          \path[-stealth, auto]
            (m-1-1) edge (m-1-2)
            (m-2-1) edge (m-2-2)
            (m-2-1) edge[equiv1step] (m-1-1)
            (m-2-2) edge[equiv] (m-1-2);
        \end{tikzpicture} 
      \end{center}
  
  \end{itemize}

  We consider the two cases separately : let us assume that $\mathcal{R} \to
  \mathcal{R'}$ is not a duplication.
  We proceed first on induction on the length of the reduction $\mathcal{S}
  \leadsto^k \mathcal{R}$. The induction hypothesis is that we can always fill
  the following diagram

  \begin{center}
      \begin{tikzpicture}
        \matrix (m) [matrix of math nodes,row sep=3em,column sep=4em,minimum
          width=2em] 
        {
          \mathcal{R} & \mathcal{R}' \\
          \mathcal{S} & \mathcal{S'} \\
        };
        \path[-stealth, auto]
          (m-1-1) edge (m-1-2)
          (m-2-1) edge[reduceto] (m-2-2)
          (m-2-1) edge[equivkstep] (m-1-1)
          (m-2-2) edge[equivkpstep] (m-1-2);
      \end{tikzpicture} 
  \end{center}

  With $k' \leq k$ and the bottom reduction does not perform any duplication.
  The base case $k=0$ is trivially true. For the induction step, if we have
  $\mathcal{S} \leadsto^k \mathcal{T} \leadsto \mathcal{R}$, we use the first
  diagram of the remarks to get the middle line $T \to^\ast T_p$.  Then, we
  apply the induction hypothesis on each reduction step $T_i \to T_{i+1}$, which
  we can do precisely because our IH states that the length $k_i$ of each
  reduction $S_i \leadsto^{k_i} T_i$ verifies $k_i \leq k_{i-1} \leq \ldots \leq
  k$. We paste all the diagrams and get 

  \begin{center}
      \begin{tikzpicture}
        \matrix (m) [matrix of math nodes,row sep=3em,column sep=1em,minimum
          width=1em] 
        {
          \mathcal{R} & & & \mathcal{R}' \\
          \mathcal{T} & \mathcal{T}_1 & \phantom{|}\ldots & \mathcal{T}_p \\
          \mathcal{S} & \mathcal{S}_1 & \phantom{|}\ldots & \mathcal{S}_p \\
        };
        \path[-stealth, auto]
          (m-1-1) edge (m-1-4)
          (m-2-1) edge (m-2-2)
          (m-2-2) edge (m-2-3)
          (m-2-3) edge (m-2-4)
          (m-3-1) edge (m-3-2)
          (m-3-2) edge (m-3-3)
          (m-3-3) edge (m-3-4)
          (m-2-1) edge[equiv1step] (m-1-1)
          (m-2-4) edge[equiv01step] (m-1-4)
          (m-3-1) edge[equiv] (m-2-1)
          (m-3-2) edge[equiv] (m-2-2)
          (m-3-4) edge[equiv] (m-2-4);
      \end{tikzpicture} 
  \end{center}

  The case of duplication is simpler as the step $\mathcal{R} \to \mathcal{R}'$
  is reflected by just one step $\mathcal{S} \to \mathcal{S}'$ in the second
  diagram of the remarks. Our IH is just that we can fill the diagram, without
  further assertion on the length of the $\leadsto$ reduction. Indeed, if $\mathcal{S} \leadsto^k \mathcal{T}
  \leadsto \mathcal{R}$, we use the one-step diagram to get $\mathcal{T}'$ and
  the IH to fill the bottom part with $\mathcal{S}'$ : 

  \begin{center}
      \begin{tikzpicture}
        \matrix (m) [matrix of math nodes,row sep=3em,column sep=4em,minimum
          width=2em] 
        {
          \mathcal{R} & \mathcal{R}' \\
          \mathcal{T} & \mathcal{T}' \\
          \mathcal{S} & \mathcal{S}' \\
        };
        \path[-stealth, auto]
          (m-1-1) edge (m-1-2)
          (m-2-1) edge (m-2-2)
          (m-3-1) edge (m-3-2)
          (m-2-1) edge[equiv1step] (m-1-1)
          (m-3-1) edge[equivkstep] (m-2-1)
          (m-2-2) edge[equiv] (m-1-2)
          (m-3-2) edge[equiv] (m-2-2);
      \end{tikzpicture} 
  \end{center}

  Finally, we can perform a second induction on the length of the reduction
  $\mathcal{R} \to^\ast \mathcal{R}'$ to get the final result.
\end{proof}

\subsection{Standardization (Lemma~\ref{lemma-nets-standardization})}

\begin{proof}\ref{lemma-nets-standardization}
This follows from the previous lemma: we decompose the reduction $\net R
\to^\ast S$ as blocks $\net R \leadsto^\ast R_1 \red{\text{diff}}^\ast R_2
\leadsto^\ast \ldots \red{\text{diff}}^\ast R_n$, and iterate
\ref{lemma-nets-swapping} to regroup the reductions into only two distinct
blocks.
\end{proof}

\subsection{Termination (Theorem~\ref{theorem-nets-termination})}

The following remark is needed to prove the theorem. It follows immediatly from
the observation that $\red{\text{diff}}$ only acts on surface, while $\leadsto$
reduces inside boxes, hence the latter can't interact with the former's
redexes.

\begin{lemma}{Neutrality of $\leadsto$}\label{lemma-nets-leadsto-neutrality}\\
  $\leadsto$ does not create nor erase $\red{\text{diff}}$-redexes. In
  particular, if $\net R \leadsto^\ast \net{R}'$, then $\net{R}$ is
  $\red{\text{diff}}$-normal if and only if $\net{R}'$ is.
\end{lemma}

\begin{proof}\ref{theorem-nets-termination}
\begin{itemize}
  \item $\to$-weakly normalizing implies $\red{\text{diff}}$-weakly normalizing
    \\
    Let $\net R$ be $\to$-weakly normalizing, $\net R \to^\ast \net N$ a
    reduction to its normal form. By \ref{lemma-nets-standardization}, we can write
    $\net R \red{\text{diff}}^\ast \net S \leadsto^\ast N$. $N$ being a
    $\to$-normal form, it is also a $\red{\text{diff}}$-normal form, and by
    \ref{lemma-nets-leadsto-neutrality} so is $\net S$. $\net R$ is thus a
    $\red{\text{diff}}$-weakly normalizing.
  \item an infinite $\to$-reduction gives an infinite
    $\red{\text{diff}}$-reduction\\
    Let $\net R$ be a net with an infinite reduction, noted $\net R \to^\ast
    \infty$. We will prove by induction that for any $n \geq 0$, there exists
    $\net{R}_n$ such that $R \red{\text{diff}}^n \net{R}_n \to^\ast \infty$.
    \begin{itemize}
      \item Case $n = 0$\\
        We just take $\net{R}_0 = \net R$
      \item Inductive case\\
        If $\net R \red{\text{diff}}^n \net{R}_n \to^\ast \infty$, we take any
        infinite reduction starting from $\net{R}_n$. If the first step is
        $\net{R}_n \red{\text{diff}} \net S$, then we take $\net{R}_{n+1} = \net
        S$. Otherwise, the first step is $\leadsto$ one, and we take the maximal
        block of $\leadsto$ reduction starting from $\net{R}_n$. By \ref{}, this block must indeed be
        finite and we can write $\net{R}_n \leadsto^\ast \net S
        \red{\text{diff}} \net{S}'$. By \ref{lemma-nets-swapping}, we can swap the
        two blocks such that $\net{R}_n \to \net{R}' \to^\ast \net{R}''
        \leadsto^\ast \net{S}'$, and we take $\net{R}_{n+1} = \net{R}'$.
    \end{itemize}
\end{itemize}
From these two points follows that $\to$-weak normalization implies $\to$-strong
normalization.
\end{proof}

\section{Routing}
\label{appendix:routing}

\begin{definition}{Arity}\label{appendix-routing-arity}\\
Let $(\labin, \labout, R)$ be a routing area. For an input $i \in \labin$, we
define its \emph{arity} as the number of leafs of the associated contraction
tree given by $\arity{i} = \sum_{o \in \labout} R(i,o)$. Similarly, the arity of
an output $o \in \labout$ is defined by $\arity{o} = \sum_{i \in \labin}
R(i,o)$. The set of outputs (resp. inputs) connected to an input $i$ (resp.
output $o$) is defined as $\conn{i} = \{ o \in \labout \mid R(i,o) \geq 1 \}$
(resp. $\conn{o} = \{ i \in \labin \mid R(i,o) \geq 1 \}$). In general, for an
input or an output $x$, $\arity{x} \leq \cardn{\conn{x}}$.  This is an equality
for all $x$ if and only if $R$ is a relation.
\end{definition}

\subsection{Trace (Property~\ref{property-mrarea-trace})}

\begin{proof}\ref{property-mrarea-trace}
  If $\arity{i} = \arity{o} = 0$, then we connected a coweakening to a weakening
  and we can erase them to recover the desired area where $T$ is just the
  restriction of $R$ to $(\labin - \{i\}) \times (\labout - \{o\})$, which
  agrees with the formula of \ref{property-mrarea-trace} as the product
  $R(x,o)R(i,y)$ is always zero.

  Now, assume that $\arity{o} = 0 < \arity{i}$. We can reduce the introduced
  redex as follow :
\begin{center}
  \tikzvcenter{
    \begin{proofnet}
      % Tree of i1
      \init[grow=left]{
        \zeroary[normal,name=i1]{\oc}
      }
      % Tree of im
      \init[grow=right]{
        \nary[name=im]{\wn}{
          \wire{\point(im1)},
          \point(im2),
          \wire{\point(im3)}
        }
      }
      \pdots[2pt](i11)(i13)
      \pdots[2pt](im1)(im3)
      % \pdots[5pt](i1.pal)(im.pal)
      % \pdots[2pt](o11)(o13)
      % \pdots[2pt](on1)(on3)
      % \pdots[5pt](o1.pal)(on.pal)
    \end{proofnet}  
    $\to^\ast$
    \begin{proofnet}
      % Tree of o1
      \init[grow=left]{
        \zeroary[normal,name=o1]{\oc}
      }
      % Tree of on
      \init[grow=left]([yshift=7.5ex,xshift=5pt]o1.pal){
        \zeroary[normal,name=on]{\oc}
      }
      \pdots[5pt](o1.pal)(on.pal)
    \end{proofnet} 
  }
\end{center}

These coweakening are connected to the trees of the outputs $\conn{i}$.
These are either connected to a wire, or a
cocontraction tree and we can eliminate superfluous coweakening using the equivalence
relation. Once again, we didn't create new paths and recover an area whose
relation is the restriction of $R$, still agreeing with the formula as
$\arity{i} = 0$ implies $R(x,o)R(i,y)$ being zero again. The dual case $\arity{i} = 0 <
\arity{o}$ is treated the same.
 
The general case relies on the commutation of contractions and cocontractions
trees that can be derived by iterating the corresponding reduction rule. We can apply the
following reduction on the trees of $i$ and $o$ that have been connected :

\begin{center}
  \includegraphics{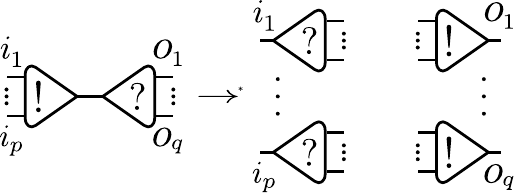}
\end{center}

where wires $i_1,\ldots,i_p$ are connected to the trees of the inputs in
$\conn{o}$ and $o_1,\ldots,o_q$ to the trees of the outputs of $\conn{i}$. The
reduced net now have the form of a routing area. As before, the direct
paths between $x$ and $y$ when $x \neq i$ and $y \neq o$ are left unchanged. But
any couple of paths in $R$ between $x$ and $o$ arriving at some $i_k$ and
between $i$ and $y$ arriving at $o_l$ yields exactly one new path between $x$
and $y$ in the new area (see \ref{property-mrarea-path-preservation} below). By
definition, there are $R(x,o)$ paths connecting $x$ to $o$ and $R(i,y)$
connecting $i$ to $y$ : hence there are $R(x,o)R(i,y)$ such couples.
\end{proof}

\subsection{Routing areas characterization
  (Theorem~\ref{theorem-mrarea-charact})}

\begin{proof}\ref{theorem-mrarea-charact}\\
 We prove the result by induction on the number $n$ of cells of $\net R$.
 \begin{itemize}
   \item ($n=0$) $\net R$ is only composed of free wires. We take $\labin = \{
     s(w) \mid w \mbox{ wire }\}$, $\labout = \{ e(w) \mid w \mbox{ wire } \}$
     and $R$ is the relation defined by $i \mathrel R o \iff \exists w,\ i =
     s(w), o = e(w)$.
   \item (induction step) Let take any node $N$ of $\net R$. We call
     $\net{R}'$ the subnet obtained by removing $N$ and replacing its ports by
     free ports.

    \begin{center}
      \includegraphics{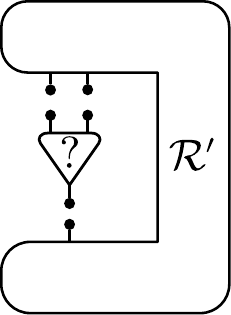}
    \end{center}

    By induction, $\net{R}'$ can be reduced to a routing area
    $\routarea{R}'$.

     \begin{description}
       \item[(co)weakening] If $N$ is a weakening or coweakening, it is a
         routing area and can be composed with $\routarea{R}'$, and reduced to a
         new routing area $\routarea{R}$ according to \ref{mcor-mrarea-merge}. Thus we can
         reduce the whole net to $\routarea{R}$. 
       \item[(co)contraction] If $N$ is a contraction or a cocontraction, it can
         still be seen as a routing area and we juxtapose it to $\routarea{R}'$.
         What remains to do is to perform three traces operations to recover the
         original net and reduce the whole net to a routing area
         $\routarea{R}$. However, we must ensure that the input and the output
         we connect at each step are not already connected in the routing
         area. The first operation is always legal, as it is actually a merge
         operation of previously disjoint areas. The following traces are also
         valid, as reduction does not create cycles, as implied by
         \ref{property-mrarea-path-preservation}. 
     \end{description}
 \end{itemize}
\end{proof}

\subsection{More on paths in routing nets}
\label{appendix:routing:paths}

Paths are barely mentionned in Theorem~\ref{theorem-mrarea-pathsemantic}. We define
them and give the fundamental properties leading to the theorem.

\begin{definition}{Paths}\label{definition-mrarea-paths}\\
  Let $\net R$ be a net. We recall that for a cell $c$ of $\net R$, we write
  $p_i(c)$ for its $i$-th auxiliary port (if it exists) and $p(c)$ for its main
  port. For a wire $w$, $s(w)$ designates the source port of $w$ while $e(w)$
  is its end port.
  Let $\net R$ be a net without exponential boxes, we construct the associated
  undirected graph $G(\net R)$ with ports as vertices and: 
  \begin{description}
    \item[Wire edges] For any wire $w$ of $\net R$, we add an edge between $s(w)$
      and $e(w)$.
    \item[Cell edges] For every auxiliary port $p_i(c)$ of a cell, we add an edge between $p_i(c)$ and $p(c)$.
  \end{description}
  A path $p$ in $\net R$ is a finite sequence
  $(p_1,e_1,p_2,e_2,\ldots,e_n,p_{n+1})$ such that $p_i$ is a port of $\net R$,
  $e_i$ an edge of $G(R)$ linking $p_i$ and $p_{i+1}$ and such that $e_i$ and
  $e_{i+1}$ are of distinct nature (cell/wire edge). We extend $s$ and $e$ to operate on path, defined by
  $s(p) = p_1$ and $e(p) = p_{n+1}$. Paths whose starting and ending edges are wire edges
  can also be described as a sequence of corresponding wires $(w_1,\ldots,w_m)$
  as internal ports and cell edges can be recovered.  We note $P(\net R)$ the
  set of paths in $\net R$ and $P_f(\net R)$ the paths starting and ending on
  free ports. 
\end{definition}

Albeit close, paths as defined here and paths of a switching graphs do not
correspond exactly. For example, a path in a switching graph can arrive at a
cocontraction premise and bounce back in the other. Our path can not. However,
the important point is that being correct and not having a cyclic paths is
actually equivalent:

\begin{property}{Acyclicity of correct nets}\label{property-mrarea-path-switching}\\
  A routing net is acyclic, that is there is no path $p$ such that $s(p) = t(p)$.
\end{property}

\begin{proof}\ref{property-mrarea-path-switching}\\
  We prove that the existence of a cycle implies the existence of a cycle in a
  switching graph.  For any subsequence $(p,e,p')$ of a path, we define its
  orientation as follows. It is $1$ when $(p,p')$ are respectively:
  \begin{itemize} \item The auxiliary and the principal port of a contraction
    cell \item The principal and the auxiliary port of a cocontraction cell
  \item The principal port of a contraction cell and the principal port of a
    cocontraction cell \item The auxiliary port of cocontraction cell and the
    auxiliary port of a contraction cell \end{itemize} and defined to be $0$ in
    all other cases, which are dual of these. This orientation is actually
    constant along a path: if we start by going from the auxiliary port to the
    principal port of a contraction cell for example, we are constrained to
    continue this way along the contraction tree until we meet a cocon tree,
    where we go in the inverse way.

  Hence, in a minimal cycle, a cell can't be visited by both its auxiliary
  ports, and this cycle is also a cycle in a switching graph.
\end{proof}

We now state a fundamental property relating reduction to paths:

\begin{property}{Path preservation}\label{property-mrarea-path-preservation}\\
  Let $\net R$ be a routing net, $p_1$ and $p_2$ be free ports. We write
  $P_f(\net R,p_1,p_2) = \{
  p \in P_f(\net R) \mid s(p) = p_1, e(p) = p_2 \}$. If $\net R \to
  \net{R}'$, then $P_f(\net R,p_1,p_2) = P_f(\net{R}',p_1,p_2)$. In particular,
  $P_f(\net R) = \sum P_f(\net R,p_i,p_{i'}) = P_f(\net{R}')$.
\end{property}

\begin{proof}\ref{property-mrarea-path-preservation}
  The proof is simple in the case of routing nets. As a path in $P_f(R,p_1,p_2)$
  must begin and end in a free port, it can't go through a weakening or a
  coweakening, and the corresponding reductions leave the paths unchanged. The
  only relevant reduction is the bialgebra rule :
  SCCHEMA
  A path either does not go through the redex, and is left unchanged in
  $\net{R}'$. Otherwise, any section of the form blah is replaced in $\net{R}'$
  by the corresponding blah.
\end{proof}

We can now prove Theorem~\ref{theorem-mrarea-pathsemantic}:

\begin{proof}\ref{theorem-mrarea-pathsemantic}
  \begin{itemize}
    \item For normal forms, this follows from the very definition of a
      routing area associated to the multirelation $\sem{\net S}$ :
      $\sem{\net S}(i,o)$ counts precisely the number of paths starting
      at port $i$ and ending at port $o$.
    \item Otherwise, by path preservation (\ref{property-mrarea-path-preservation}), this
      quantity is invariant by reduction. We conclude by induction on the length
      of the longest reduction of $\net S$ to its normal form.
  \end{itemize}
\end{proof}
